# Supplementary material for: Language Conditioned Traffic Generation
Source: arXiv:2307.07947 source file (2023-07-16)
Supplement: Supplementary file 1 [file train_pipeline.tex]

% \begin{figure*}[!t]
% \centering
% % \vspace{-5em}
% \includegraphics[width=1.0\linewidth]{supp/figures/train_pipeline_fig.pdf}
% % \vspace{-3em}
% % \caption{Instructional editing on a real-world scenario}
% % \vspace{-1em}
% \label{fig:edit_2}
% \end{figure*}
